# Supplementary material for: Seeing Isn't Orienting: A Cognitively Informed Hierarchical Benchmark for Object Orientation in MLLMs
Source: arXiv:2505.21649 source file (2026-07-12)
Supplement: Supplementary file 1 [file dori_vqa_samples.pdf]

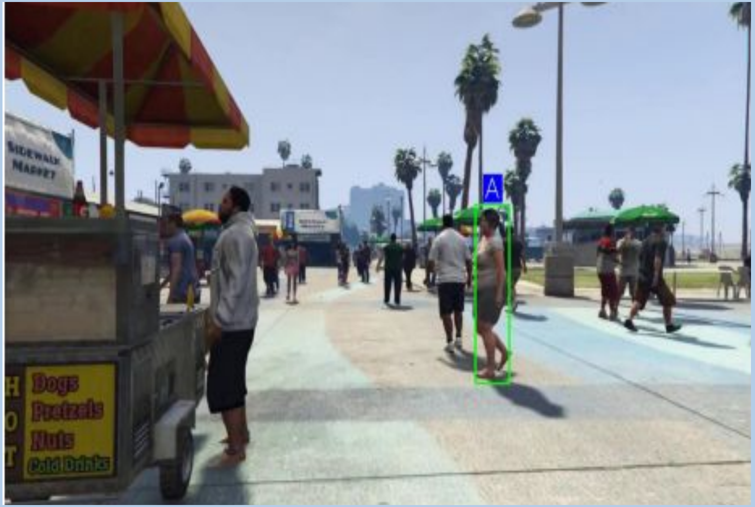


**Ground Truth:**

C: Facing away from the camera

**Gemini_1.5_pro Answer:**

"answer": "B",

"reasoning": "Object A is a person. The key structural feature for a person is their face. We can see her face clearly and we can tell her body is oriented towards the camera, therefore Object A is facing directly towards the camera."

**Prompt:**

TASK: Determine which way Object A's front is facing relative to the camera.

CONTEXT: Object A is marked with a bounding box in the image. An object is considered 'front facing' when its inherent structural features (e.g., a person's face, car headlights, TV screen) are visible from the camera.

Please analyze this image using these steps:
1. Identify Object A and its key structural features 2. Determine the orientation of its front surface relative to the camera 3. Compare with the provided options 4. Select the most appropriate answer 5. Explain your reasoning with specific visual evidence

OPTIONS:
A. Not visible enough to determine B. Directly facing the camera
C. Facing away from the camera

FORMAT YOUR RESPONSE AS:
"answer": "Letter/number of chosen option",
"reasoning": "Step-by-step explanation citing specific visual evidence"

EXAMPLES:
- A person whose body is directed towards the camera would be "facing toward the camera"

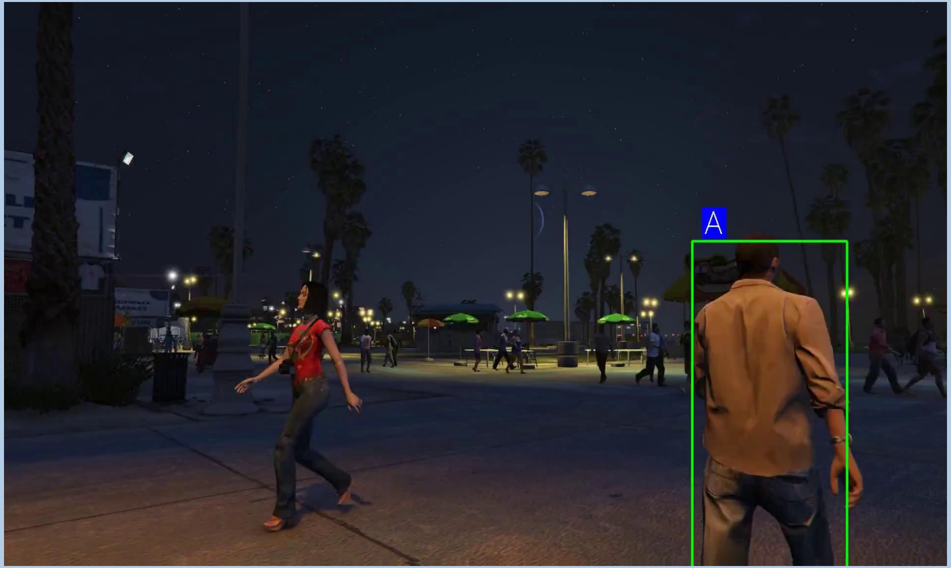


**Ground Truth:**

A : 135 degrees to 180 degrees

**Gemini-2.0-Flash Answer:**

"Answer": "B",

"Reasoning": "Object A's back is to the camera. Therefore, the deviation from the camera plane is between 0 degrees and 15 degrees."

**Prompt:**

TASK: Determine how much Object A's front surface deviates from being parallel to the camera plane.

CONTEXT: Object A is marked with a bounding box in the image. You'll be assessing the angle between Object A's front surface and the camera plane (the camera taking this photo). Please analyze this image using these steps: 1. Identify Object A and establish its front-facing surface 2. Estimate the angular deviation between this surface and the camera plane 3. Compare with the provided options 4. Select the most appropriate answer 5. Explain your reasoning with specific visual evidence

OPTIONS: A. 135 degrees to 180 degrees B. 0 degrees to 15 degrees C. Cannot be determined D. 65 degrees to 95 degrees

FORMAT YOUR RESPONSE AS: "answer": "Letter/number of chosen option", "reasoning": "Step-by-step explanation citing specific visual evidence" EXAMPLES: - A person looking directly at the camera: 0-15 degrees - A person is perpendicular to the camera: 65-95 degrees - A car with its rear-end to the camera: 135-180 degrees

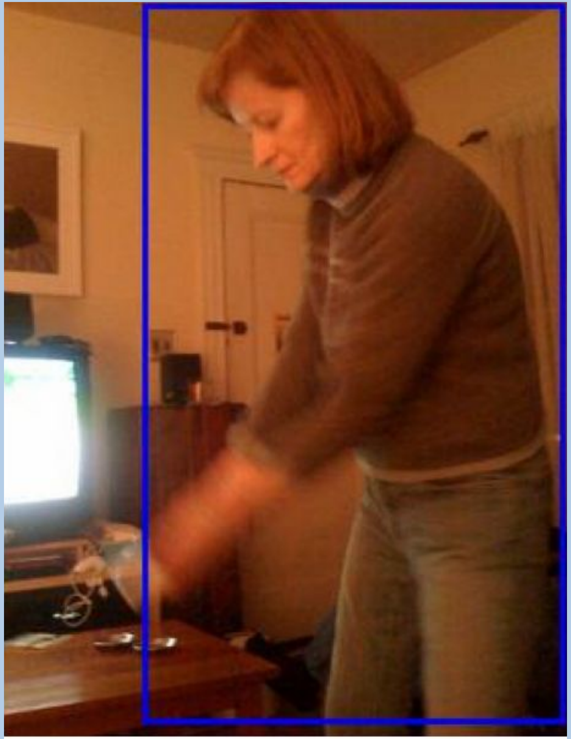

**Prompt:**

TASK: Determine which direction Object A's front-facing surface is oriented from the camera's viewpoint.

CONTEXT: Object A is marked with a bounding box in the image. You will identify its front-facing surface orientation based on inherent structural features.Please analyze this image using these steps:1. Identify Object A and establish its front-facing surface 2. Determine the direction this surface is oriented relative to the camera3. Compare with the provided options 4. Select the most appropriate answer 5. Explain your reasoning with specific visual evidence

OPTIONS:{'A': 'Toward the camera' 'B': "Can't be determined" 'C': 'Away from the camera' 'D': 'Rightward relative to the camera plane' 'E': 'Leftward relative to the camera plane'}

FORMAT YOUR RESPONSE AS: "answer": "Letter/number of chosen option" "reasoning": "Step-by-step explanation citing specific visual evidence"

EXAMPLES:- If you see a car with its headlights directly pointing toward the camera select "Toward the camera"- If you see a person with their back to the camera select "Away from the camera"

**Ground Truth:**

E: Leftward relative to the camera plane

**Gpt_4_1 Answer:**

Answer: "B"

"reasoning": "The person inside the bounding box (Object A) is facing away from the camera. This is evident because the back of their head and body are visible while their face is not. The orientation of the shoulders and the direction of the arms also indicate that the front-facing surface (the person's face and torso) is directed away from the camera."

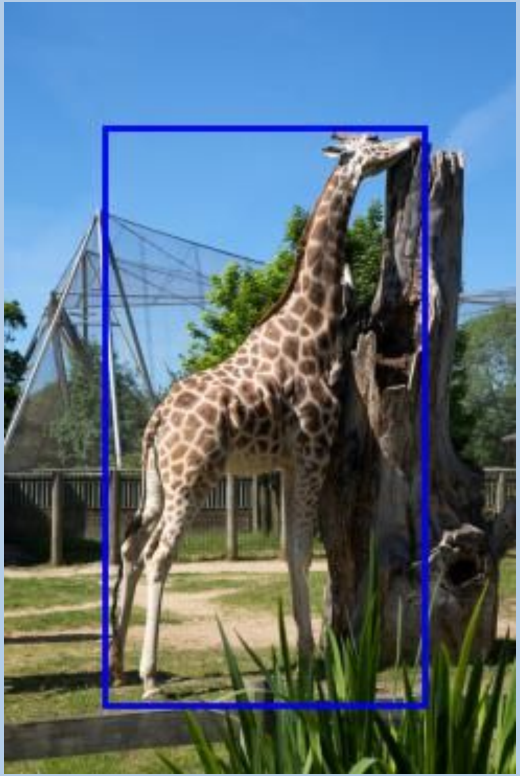

**Prompt:**

TASK: Determine which direction Object A's front-facing surface is oriented from the camera's viewpoint.

CONTEXT: Object A is marked with a bounding box in the image. You will identify its front-facing surface orientation based on inherent structural features. Please analyze this image using these steps: 1. Identify Object A and establish its front-facing surface 2. Determine the direction this surface is oriented relative to the camera 3. Compare with the provided options 4. Select the most appropriate answer 5. Explain your reasoning with specific visual evidence

OPTIONS: A. Can't be determined B. Rightward relative to the camera plane C. Away from the camera D. Toward the camera E. Leftward relative to the camera plane FORMAT YOUR RESPONSE AS: "answer": "Letter/number of chosen option", "reasoning": "Step-by-step explanation citing specific visual evidence"

EXAMPLES: - If you see a car with its headlights directly pointing toward the camera, select "Toward the camera" - If you see a person with their back to the camera, select "Away from the camera"

**Ground Truth:**

B : Rightward relative to the camera plane

**Gemini-2.0-Flash Answer:**

"Answer": "E",

"Reasoning": "The giraffe in the image (Object A) is oriented so that its front-facing surface (as indicated by its face, neck, and body) is primarily directed leftward relative to the camera's perspective. This is because the giraffe is largely facing towards the left side of the image."

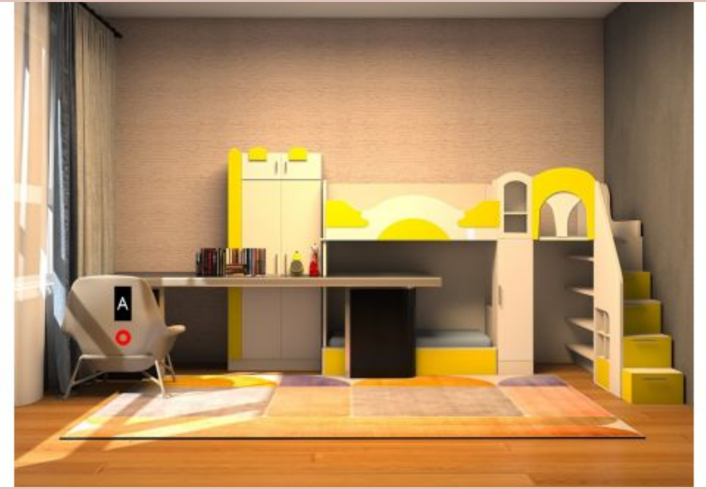


**Ground Truth:**

E: 180 degrees

**GPT-4O Answer:**

“Answer": "E"
"reasoning": "The object marked as 'A' is a chair and it does not have a clear front-facing surface that can be definitively identified. Without a clear indication of its front orientation it is impossible to determine how many degrees of clockwise rotation would be needed for it to face the camera. Therefore the correct answer is 'Cannot be determined.”

**Prompt:**

TASK: Determine the closest clockwise rotation needed for Object A to face the camera.

CONTEXT: Object A is marked with a bounding box in the image. Objects can rotate clockwise or counterclockwise around a vertical axis (running from top to bottom).Please analyze this image using these steps: 1. Identify Object A and establish its front-facing surface 2. Determine its current orientation relative to the camera3. Calculate how many degrees of clockwise rotation would be needed to make it face the camera4. Compare with the provided options 5. Select the most appropriate answer 6. Explain your reasoning with specific visual evidence

OPTIONS:{'A': '0 degrees' 'B': '90 degrees' 'C': '45 degrees' 'D': '135 degrees' 'E': '180 degrees' 'F': 'Cannot be determined'} FORMAT YOUR RESPONSE AS:"answer": "Letter/number of chosen option" "reasoning": "Step-by-step explanation citing specific visual evidence"

EXAMPLES:- If the object is already facing the camera the answer is "0 degrees"- If the object's front is facing to your right a "90 degrees" clockwise rotation would make it face the camera- If the object's front is at a 45-degree angle to your right a "45 degrees" clockwise rotation would make it face the camera- If the object's front is at a 135-degree angle to your right a "135 degrees" clockwise rotation would make it face the camera- If the object's front is facing away from the camera a "180 degrees" clockwise rotation would make it face the camera- If the object has no clear front or its orientation cannot be determined select "Cannot be determined"

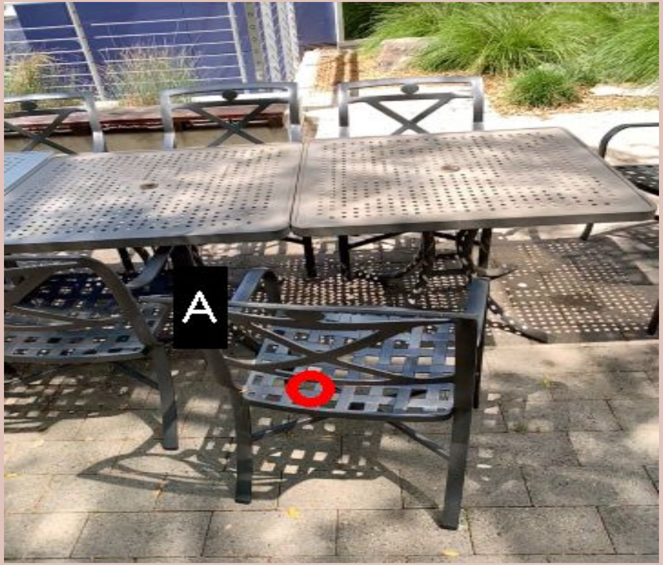


**Ground Truth:**

E: 180 degrees

**Gemini-2.0-Flash Answer:**

"Answer": "B",

"Reasoning": "Object A is currently oriented approximately 90 degrees clockwise from facing the camera. A clockwise rotation of 90 degrees would be needed to make it directly face the camera."

**Prompt:**

TASK: Determine the closest clockwise rotation needed for Object A to face the camera.

CONTEXT: Object A is marked with a bounding box in the image. Objects can rotate clockwise or counterclockwise around a vertical axis (running from top to bottom). Please analyze this image using these steps: 1. Identify Object A and establish its front-facing surface 2. Determine its current orientation relative to the camera 3. Calculate how many degrees of clockwise rotation would be needed to make it face the camera 4. Compare with the provided options 5. Select the most appropriate answer 6. Explain your reasoning with specific visual evidence

OPTIONS: A. 0 degrees B. 90 degrees C. 45 degrees D. Cannot be determined E. 180 degrees F. 135 degrees FORMAT YOUR RESPONSE AS: "answer": "Letter/number of chosen option", "reasoning": "Step-by-step explanation citing specific visual evidence"

EXAMPLES: - If the object is already facing the camera, the answer is "0 degrees" - If the object's front is facing to your right, a "90 degrees" clockwise rotation would make it face the camera - If the object's front is at a 45-degree angle to your right, a "45 degrees" clockwise rotation would make it face the camera - If the object's front is at a 135-degree angle to your right, a "135 degrees" clockwise rotation would make it face the camera - If the object's front is facing away from the camera, a "180 degrees" clockwise rotation would make it face the camera - If the object has no clear front or its orientation cannot be determined, select "Cannot be determined"

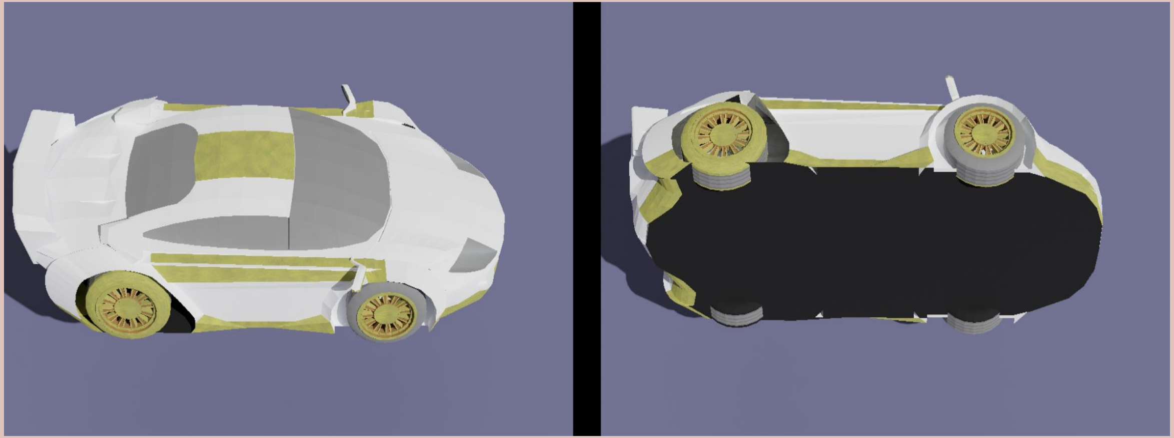

**Gemini-2.0-Flash Answer:**

"Answer": "C",

"Reasoning": "The car in the first image is upright with the wheels on the bottom. In the second image, the car is upside down with the undercarriage showing. This indicates a rotation around a horizontal axis."

**Prompt:**

TASK: Determine what type of rotation the object has undergone between the two images.

CONTEXT: Two images of the same object are shown side by side. The object can rotate around two axes: Horizontal (like a cartwheel coming out of the screen) and Vertical (like a ballerina spinning clockwise). Please analyze these images using these steps: 1. Identify the object in both images and establish its key features 2. Compare the object's orientation in both images 3. Determine which axes the object has rotated around 4. Compare with the provided options 5. Select the most appropriate answer 6. Explain your reasoning with specific visual evidence

OPTIONS: A. Cannot be determined B. Only Vertical C. Only Horizontal D. Both Horizontal and Vertical E. No Change FORMAT YOUR RESPONSE AS: "answer": "Letter/number of chosen option", "reasoning": "Step-by-step explanation citing specific visual evidence"

EXAMPLES: - If an object appears to have moved to face left or right between images, select "Only Vertical" - If an object appears to have moved up or down (like nodding), select "Only Horizontal" - If an object has rotated both horizontally and vertically, select "Both Horizontal and Vertical" - If the object appears identical in both images with no rotation, select "No Change" - If you cannot clearly determine the type of rotation, select "Cannot be determined"

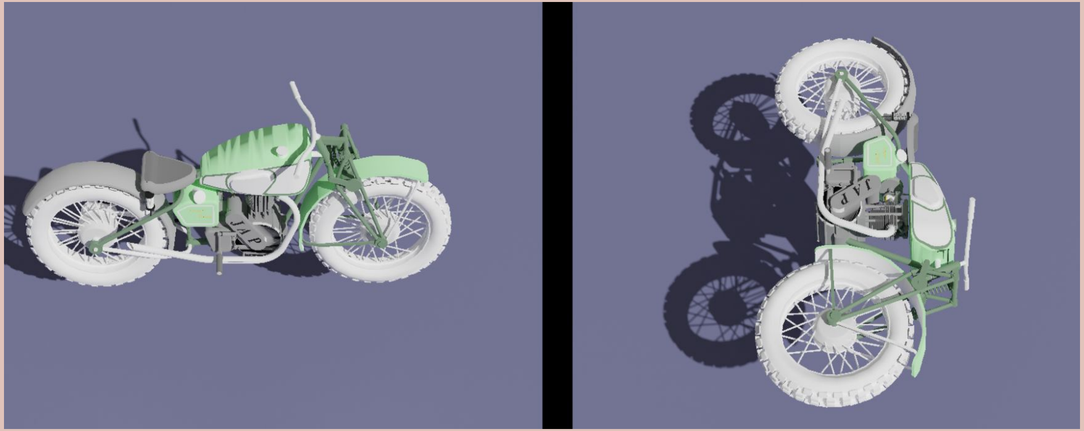

**Ground Truth:**
E: 90 Degrees Horizontal, 90 Degrees Vertical

**Gemini-2.0-Flash Answer:**

"Answer": "E",

"Reasoning": "The motorcycle in the first image is upright. In the second image, the motorcycle is rotated 90 degrees horizontally, leaning to the right. Additionally, it has been rotated 180 degrees vertically, as evidenced by the seat and rear tire now facing upward."

**Prompt:**
TASK: Determine the exact rotation angles the object has undergone between the two images.

CONTEXT: Two images of the same object are shown side by side. The object can rotate around two axes: Horizontal (like a cartwheel coming out of the screen) and Vertical (like a ballerina spinning clockwise). Please analyze these images using these steps: 1. Identify the object in both images and establish its key features 2. Compare the object's orientation in both images 3. Determine the horizontal rotation angle first, then the vertical rotation angle 4. Compare with the provided options 5. Select the most appropriate answer 6. Explain your reasoning with specific visual evidence

OPTIONS: A. 270 degrees Horizontal then 180 degrees Vertical B. 180 degrees Horizontal then 0 degrees Vertical C. Cannot be determined D. 180 degrees Horizontal then 90 degrees Vertical E. 90 degrees Horizontal then 180 degrees Vertical F. 0 degrees Horizontal then 0 degrees Vertical G. 270 degrees Horizontal then 90 degrees Vertical H. 270 degrees Horizontal then 270 degrees Vertical I. 0 degrees Horizontal then 90 degrees Vertical J. 180 degrees Horizontal then 270 degrees Vertical K. 0 degrees Horizontal then 180 degrees Vertical L. 0 degrees Horizontal then 270 degrees Vertical M. 90 degrees Horizontal then 0 degrees Vertical N. 90 degrees Horizontal then 270 degrees Vertical O. 90 degrees Horizontal then 90 degrees Vertical P. 180 degrees Horizontal then 180 degrees Vertical Q. 270 degrees Horizontal then 0 degrees Vertical

FORMAT YOUR RESPONSE AS: "answer": "Letter/number of chosen option", "reasoning": "Step-by-step explanation citing specific visual evidence"

EXAMPLES: - If an upright cup in the first image appears upside-down in the second image, this might be "180 degrees Horizontal then 0 degrees Vertical" - If a car facing left in the first image appears to be tilted upward and facing the camera in the second image, this might be "90 degrees Horizontal then 90 degrees Vertical" - If you cannot clearly determine the type of rotation, select "Cannot be determined"

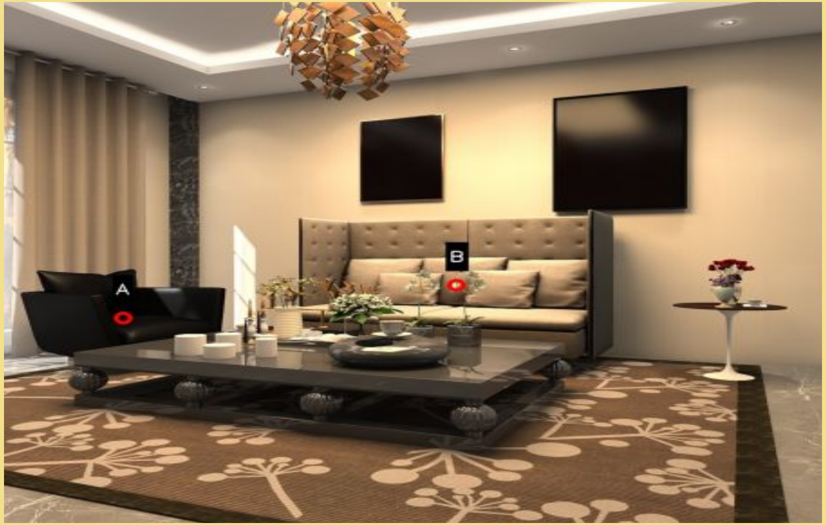


**Ground Truth:**
D: 46 to 90 degrees clockwise

**Gemini_1.5_pro Answer:**

"Answer": "F",
"reasoning": "Object A (the black chair) is facing the coffee table in the center of the room. Object B (the sofa) is currently facing the wall with the two black canvases. To face the coffee table and therefore object A, object B needs to rotate clockwise a small amount, placing it between 0 and 45 degrees. "

**Prompt:**
TASK: Determine how much Object B would need to rotate to face Object A.

CONTEXT: Objects A and B are marked with red dots in the image. You will analyze their relationship from the objects' perspectives, not from the camera view. Please analyze this image using these steps:
1. Identify objects A and B and establish their front-facing surfaces
2. Mentally position yourself at each object's location
3. Determine how much and in which direction Object B would need to rotate to face Object A
4. Compare with the provided options
5. Select the most appropriate answer
6. Explain your reasoning with specific visual evidence

OPTIONS:
A. Cannot be determined B. No rotation C. 180 degrees in either direction
D. 46 to 90 degrees clockwise E. 46 to 90 degrees counterclockwise
F. 0 to 45 degrees clockwise G. 91 to 135 degrees clockwise
H. 0 to 45 degrees counterclockwise I. 91 to 135 degrees counterclockwise

FORMAT YOUR RESPONSE AS:
"answer": "Letter/number of chosen option",
"reasoning": "Step-by-step explanation citing specific visual evidence"

EXAMPLES:
- If Object B needs to turn slightly right to match Object A's direction, select "0 to 45 degrees clockwise"
- If Object B is already facing the same direction as Object A, select "0 degrees or no rotation"
- If Object B needs to turn completely around to match Object A, select "180 degrees in either direction"

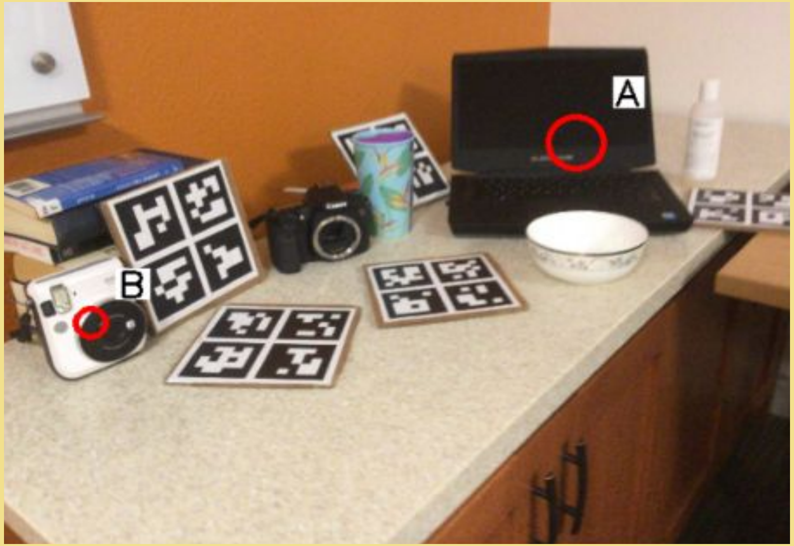


**Prompt**:

TASK: Determine if objects A and B are facing each other from their own perspectives.

CONTEXT: Objects A and B are marked with red dots in the image. You will analyze their relationship from the objects' perspectives not from the camera view.Please analyze this image using these steps: 1. Identify objects A and B and establish their front-facing surfaces 2. Mentally position yourself at each object's location 3. Determine the relative directional orientation between the objects 4. Compare with the provided options 5. Select the most appropriate answer 6. Explain your reasoning with specific visual evidence

OPTIONS:{'A': 'Cannot be determined' 'B': 'Partially facing the same direction' 'C': 'Partially facing the opposite directions' 'D': 'They are facing opposite directions' 'E': 'They are facing perpendicular to each other' 'F': 'They are facing the same direction'}

FORMAT YOUR RESPONSE AS:"answer": "Letter/number of chosen option" "reasoning": "Step-by-step explanation citing specific visual evidence"

EXAMPLES:- Two people looking at each other would be "facing opposite directions" (as their faces point toward each other)- Two cars with headlights pointing the same way would be "facing the same direction"- A car and a person where the car's side faces the person's front would be "facing perpendicular to each other"- Two objects with front surfaces angled slightly toward each other would be "partially facing opposite directions"- Two objects with front surfaces angled slightly away from each other would be "partially facing the same direction"

**Ground Truth:**

B: Partially facing the same direction

**Gpt-4-1 Answer:**

Answer: "C"

"reasoning": "...the most appropriate answer is 'Partially facing the opposite directions' as their front surfaces are somewhat oriented toward each other but not directly..."

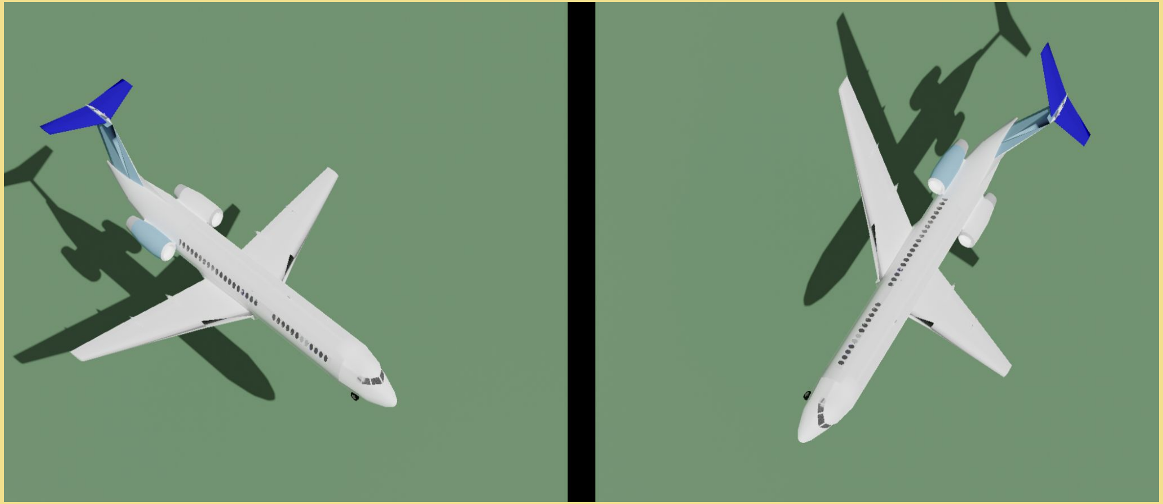

**Gemini-2.0-Flash Answer:**

"Answer": "C",

"Reasoning": "The airplane rotates 90 degrees clockwise. In the first picture, the plane's nose points towards the right, in the second picture, it points to the bottom."

**Prompt:**

TASK: Determine how many degrees clockwise the object has rotated between the two images.

CONTEXT: Two images of the same object are shown side by side. Assume the camera remains stationary, and the object can rotate around a vertical axis. Please analyze these images using these steps: 1. Identify the object in both images and establish its key features 2. Compare the object's orientation in both images 3. Determine the precise clockwise rotation angle around the vertical axis 4. Compare with the provided options 5. Select the most appropriate answer 6. Explain your reasoning with specific visual evidence

OPTIONS: A. Cannot be determined B. 180 degrees C. 90 degrees D. 270 degrees E. 0 degrees

FORMAT YOUR RESPONSE AS: "answer": "Letter/number of chosen option", "reasoning": "Step-by-step explanation citing specific visual evidence" EXAMPLES: - Objects that are symmetrical like a ball or a box would be considered "Cannot be determined

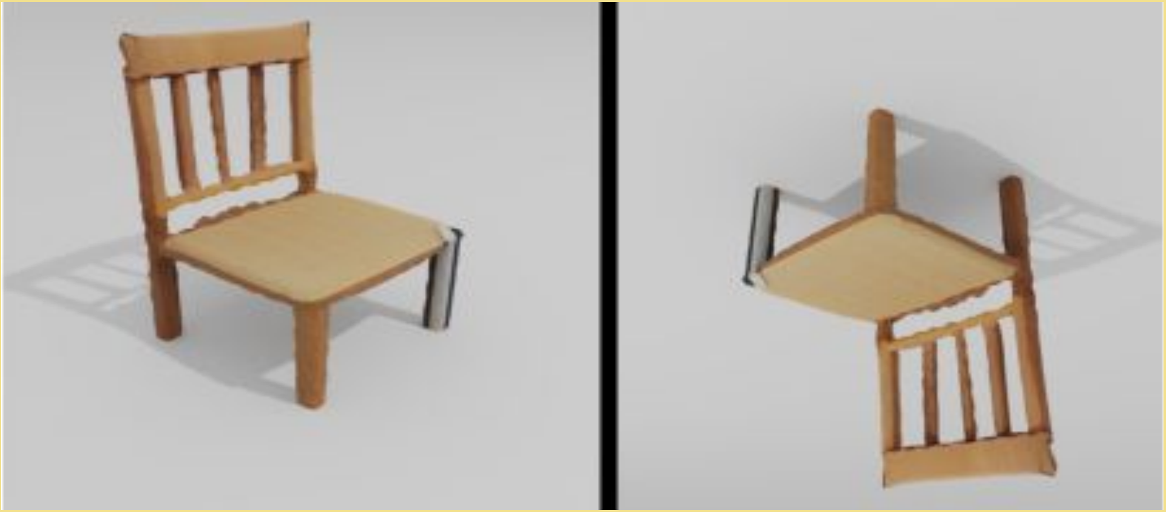

**Ground Truth:**

A: 180 degrees

**Gpt-4-1 Answer:**

Answer: "A"

"reasoning": "...Comparing the two images the chair has rotated 90 degrees clockwise around the vertical axis: the backrest moves from facing upper left to facing right ..."

**Prompt:**

TASK: Determine how many degrees clockwise the object has rotated between the two images.

CONTEXT: Two images of the same object are shown side by side. Assume the camera remains stationary and the object can rotate around a vertical axis.Please analyze these images using these steps: 1. Identify the object in both images and establish its key features 2. Compare the object's orientation in both images3. Determine the precise clockwise rotation angle around the vertical axis 4. Compare with the provided options 5. Select the most appropriate answer 6. Explain your reasoning with specific visual evidence

OPTIONS:{'A': '180 degrees' 'B': '0 degrees' 'C': '270 degrees' 'D': '90 degrees' 'E': 'Cannot be determined'}

FORMAT YOUR RESPONSE AS:"answer": "Letter/number of chosen option" "reasoning": "Step-by-step explanation citing specific visual evidence" EXAMPLES:- Objects that are symmetrical like a ball or a box would be considered "Cannot be determined"

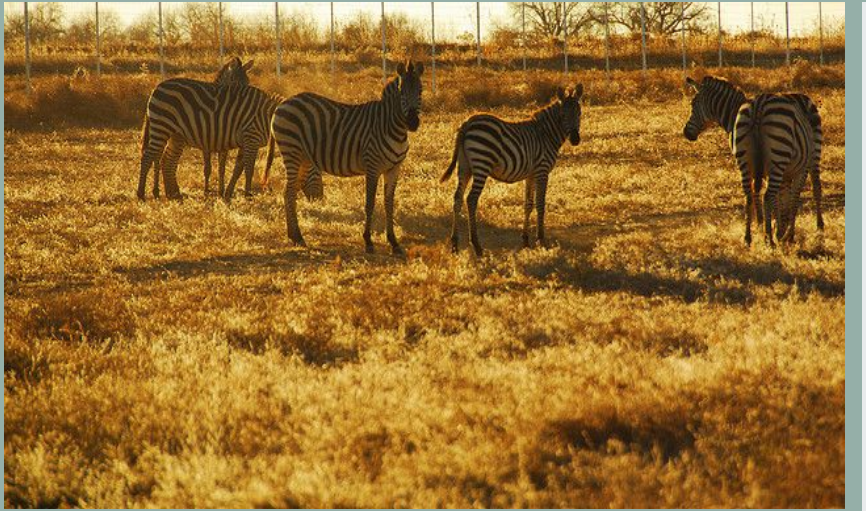

**Prompt:**

TASK: Determine how the image can be restored to its canonical orientation.

CONTEXT: The image may be flipped or rotated or both. A flipped image is mirrored horizontally or vertically. A rotated image has been turned around a point. Canonical orientation refers to the standard way objects are typically viewed. Please analyze this image using these steps: 1. Identify the main objects/elements in the image 2. Determine their expected canonical orientation 3. Analyze what transformations would restore canonical orientation 4. Compare with the provided options 5. Select the most appropriate answer 6. Explain your reasoning with specific visual evidence

OPTIONS: A. Cannot be determined B. First Flipping, and then Rotation is needed C. First Rotation, and then Flipping is needed D. No rotation or flip is needed E. Only Rotation is needed F. Only Flipping is needed

FORMAT YOUR RESPONSE AS: "answer": "Letter/number of chosen option", "reasoning": "Step-by-step explanation citing specific visual evidence"

EXAMPLES: - An upside-down book would require "Only Rotation" to restore - A mirror image of a car would require "Only Flipping" to restore - A sideways and mirrored street sign might require "First Rotation, and then Flipping" - A mirrored and then tilted building might require "First Flipping, and then Rotation" - A normally oriented landscape would require "No change needed" - An abstract pattern with no clear orientation would be "Cannot be determined"

**Gemini-2.0-Flash Answer:**

"Answer": "D.

No rotation or flip is needed",

"Reasoning":

"The zebras are standing upright, and the landscape appears normal. There is no indication that the image has been flipped or rotated. Thus, no transformation is needed to restore it to its canonical orientation."

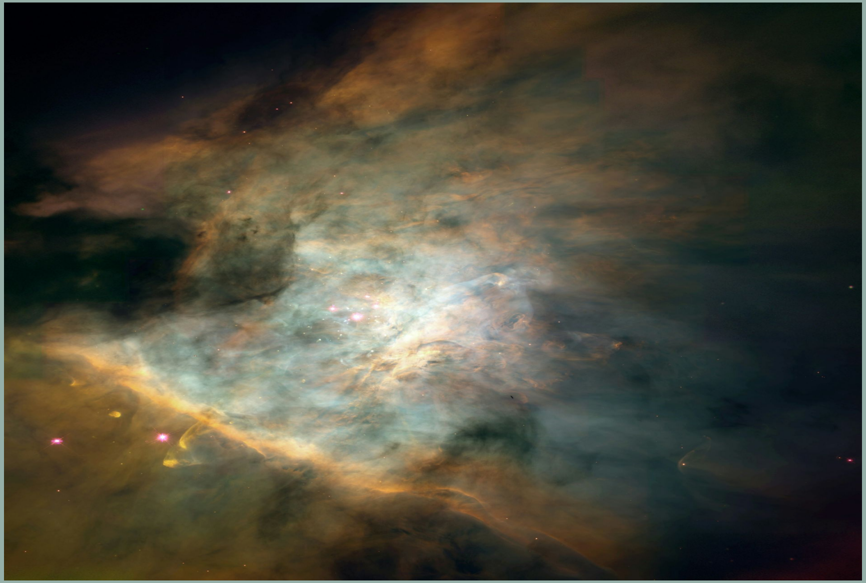

**Ground Truth:**

B. Cannot be determined

**Gemini-2.0-Flash Answer:**

"Answer": "A",

"Reasoning": "The image depicts a nebula. There is no single canonical orientation for nebulae as they are typically viewed from various angles. Therefore, the image is most likely in its canonical orientation."

**Prompt:**

TASK: Determine if the image is in its canonical orientation.

CONTEXT: The image may be flipped or rotated or both. Canonical orientation refers to the standard way objects are typically viewed (e.g., people standing upright, cars with wheels on the ground, text reading left to right).An image that has been mirrored horizontally or vertically is considered flipped. An image that has been turned from its normal viewing angle is considered rotated. Please analyze this image using these steps: 1. Identify the main objects/elements in the image 2. Determine their expected canonical orientation 3. Compare with their current orientation in the image 4. Compare with the provided options 5. Select the most appropriate answer 6. Explain your reasoning with specific visual evidence

OPTIONS: A. Yes, the image is in the canonical orientation B. Cannot be determined C. No, the image is not in the canonical orientation

FORMAT YOUR RESPONSE AS: "answer": "Letter/number of chosen option", "reasoning": "Step-by-step explanation citing specific visual evidence"
